# Supplementary material for: Frame-Semantic Parsing with Softmax-Margin Segmental RNNs and a Syntactic Scaffold
Source: arXiv:1706.09528 source file (2017-06-29)
Supplement: Supplementary file 1 [file devset.tex]

\section{Development data}
\label{sect:devset}

\begin{enumerate}
  \small
  \item \texttt{ANC\_\_110CYL072}
  \item \texttt{KBEval\_\_MIT}
  \item \texttt{LUCorpus-v0.3\_\_20000415\_apw\_eng-NEW}
  \item \texttt{LUCorpus-v0.3\_\_ENRON-pearson-email-25jul02}
  \item \texttt{Miscellaneous\_\_Hijack}
  \item \texttt{NTI\_\_NorthKorea\_NuclearOverview}
  \item \texttt{NTI\_\_WMDNews\_062606}
  \item \texttt{PropBank\_\_TicketSplitting}
\end{enumerate}
